# Supplementary material for: Learning to Select Source-Traceable Evidence for Language-Model Prediction from Irregular Clinical Time Series
Source: arXiv:2605.20292 source file (2026-09-30)
Supplement: Supplementary file 1 [file figure_concept_auroc.tex]

\begin{figure}[!htbp]
\centering
\includegraphics[width=0.3230\linewidth]{images/concept_retention_auroc_p2012.pdf}\hfill
\includegraphics[width=0.3230\linewidth]{images/concept_retention_auroc_mimic3.pdf}\hfill
\includegraphics[width=0.3230\linewidth]{images/concept_retention_auroc_p2019.pdf}
\caption{AUROC for the reader-only concept-availability intervention in Figure~\ref{fig:concept_retention}. Error bars denote standard deviation across three model seeds after averaging five draws within each seed.}
\label{fig:concept_retention_auroc}
\end{figure}
