# Supplementary material for: Learning to Select Source-Traceable Evidence for Language-Model Prediction from Irregular Clinical Time Series
Source: arXiv:2605.20292 source file (2026-09-30)
Supplement: Supplementary file 2 [file table_supp_deletion_values.tex]

% Generated from data/results_source.md by scripts/build_tables.py.
\begin{table}[!htbp]
\centering
\caption{Evidence deletion: (a) P2012 test AUPRC.}
\label{tab:deletion_auprc_p2012}\label{tab:deletion}
\footnotesize
\setlength{\tabcolsep}{1.0pt}\renewcommand{\arraystretch}{1.16}
\begin{tabularx}{\linewidth}{@{}>{\hsize=0.5385\hsize\linewidth=\hsize\raggedright\arraybackslash}X>{\hsize=1.1538\hsize\linewidth=\hsize\raggedright\arraybackslash}X>{\hsize=1.1538\hsize\linewidth=\hsize\raggedright\arraybackslash}X>{\hsize=1.1538\hsize\linewidth=\hsize\raggedright\arraybackslash}X@{}}
\toprule
Deleted $m$ & Highest margin & Lowest margin & Random (5 draws)\\
\midrule
0 & \metric{0.5274}{0.0049} & \metric{0.5274}{0.0049} & \metric{0.5274}{0.0049}\\
1 & \metric{0.5246}{0.0013} & \metric{0.5236}{0.0021} & \metric{0.5264}{0.0034}\\
2 & \metric{0.5230}{0.0033} & \metric{0.5225}{0.0037} & \metric{0.5247}{0.0044}\\
5 & \metric{0.5282}{0.0035} & \metric{0.5224}{0.0049} & \metric{0.5216}{0.0034}\\
10 & \metric{0.5154}{0.0096} & \metric{0.5146}{0.0059} & \metric{0.5185}{0.0045}\\
15 & \metric{0.4921}{0.0065} & \metric{0.5099}{0.0071} & \metric{0.5062}{0.0078}\\
20 & \metric{0.4580}{0.0016} & \metric{0.4791}{0.0118} & \metric{0.4814}{0.0124}\\
25 & \metric{0.3869}{0.0013} & \metric{0.4193}{0.0021} & \metric{0.4423}{0.0121}\\
30 & \metric{0.1697}{0.0004} & \metric{0.1697}{0.0004} & \metric{0.1697}{0.0004}\\
\bottomrule\end{tabularx}
\Note{Selection and checkpoint are frozen. Mean $\pm$ standard deviation over model seeds; random draws are averaged within each seed. Static covariates remain at all $m$.}
\end{table}
\begin{table}[!htbp]
\ContinuedFloat
\centering
\caption{Evidence deletion (continued): (b) MIMIC-III test AUPRC.}
\label{tab:deletion_auprc_mimiciii}
\footnotesize
\setlength{\tabcolsep}{1.0pt}\renewcommand{\arraystretch}{1.16}
\begin{tabularx}{\linewidth}{@{}>{\hsize=0.5385\hsize\linewidth=\hsize\raggedright\arraybackslash}X>{\hsize=1.1538\hsize\linewidth=\hsize\raggedright\arraybackslash}X>{\hsize=1.1538\hsize\linewidth=\hsize\raggedright\arraybackslash}X>{\hsize=1.1538\hsize\linewidth=\hsize\raggedright\arraybackslash}X@{}}
\toprule
Deleted $m$ & Highest margin & Lowest margin & Random (5 draws)\\
\midrule
0 & \metric{0.5025}{0.0056} & \metric{0.5025}{0.0056} & \metric{0.5025}{0.0056}\\
1 & \metric{0.4987}{0.0013} & \metric{0.4981}{0.0006} & \metric{0.4979}{0.0015}\\
2 & \metric{0.4952}{0.0061} & \metric{0.4962}{0.0002} & \metric{0.4965}{0.0005}\\
5 & \metric{0.4948}{0.0101} & \metric{0.4929}{0.0026} & \metric{0.4943}{0.0001}\\
10 & \metric{0.4864}{0.0068} & \metric{0.4867}{0.0057} & \metric{0.4873}{0.0001}\\
15 & \metric{0.4584}{0.0100} & \metric{0.4861}{0.0091} & \metric{0.4775}{0.0005}\\
20 & \metric{0.4240}{0.0025} & \metric{0.4569}{0.0125} & \metric{0.4580}{0.0036}\\
25 & \metric{0.3578}{0.0048} & \metric{0.4055}{0.0039} & \metric{0.3938}{0.0067}\\
30 & \metric{0.1176}{0.0018} & \metric{0.1176}{0.0018} & \metric{0.1176}{0.0018}\\
\bottomrule\end{tabularx}
\Note{Selection and checkpoint are frozen. Mean $\pm$ standard deviation over model seeds; random draws are averaged within each seed. Static covariates remain at all $m$.}
\end{table}
\begin{table}[!htbp]
\ContinuedFloat
\centering
\caption{Evidence deletion (continued): (c) P2019 test AUPRC.}
\label{tab:deletion_auprc_p2019}
\footnotesize
\setlength{\tabcolsep}{1.0pt}\renewcommand{\arraystretch}{1.16}
\begin{tabularx}{\linewidth}{@{}>{\hsize=0.5385\hsize\linewidth=\hsize\raggedright\arraybackslash}X>{\hsize=1.1538\hsize\linewidth=\hsize\raggedright\arraybackslash}X>{\hsize=1.1538\hsize\linewidth=\hsize\raggedright\arraybackslash}X>{\hsize=1.1538\hsize\linewidth=\hsize\raggedright\arraybackslash}X@{}}
\toprule
Deleted $m$ & Highest margin & Lowest margin & Random (5 draws)\\
\midrule
0 & \metric{0.5004}{0.0157} & \metric{0.5004}{0.0157} & \metric{0.5004}{0.0157}\\
1 & \metric{0.5023}{0.0153} & \metric{0.5022}{0.0162} & \metric{0.4995}{0.0157}\\
2 & \metric{0.4928}{0.0149} & \metric{0.5019}{0.0157} & \metric{0.4981}{0.0160}\\
5 & \metric{0.4784}{0.0218} & \metric{0.4957}{0.0153} & \metric{0.4917}{0.0170}\\
10 & \metric{0.4355}{0.0326} & \metric{0.4873}{0.0141} & \metric{0.4806}{0.0172}\\
15 & \metric{0.3888}{0.0413} & \metric{0.4703}{0.0117} & \metric{0.4619}{0.0183}\\
20 & \metric{0.3327}{0.0466} & \metric{0.4505}{0.0074} & \metric{0.4250}{0.0254}\\
25 & \metric{0.2469}{0.0385} & \metric{0.3815}{0.0086} & \metric{0.3309}{0.0295}\\
30 & \metric{0.0415}{0.0035} & \metric{0.0415}{0.0035} & \metric{0.0415}{0.0035}\\
\bottomrule\end{tabularx}
\Note{Selection and checkpoint are frozen. Mean $\pm$ standard deviation over model seeds; random draws are averaged within each seed. Static covariates remain at all $m$.}
\end{table}
\begin{table}[!htbp]
\ContinuedFloat
\centering
\caption{Evidence deletion (continued): (d) P2012 test AUROC.}
\label{tab:deletion_auroc_p2012}
\footnotesize
\setlength{\tabcolsep}{1.0pt}\renewcommand{\arraystretch}{1.16}
\begin{tabularx}{\linewidth}{@{}>{\hsize=0.5385\hsize\linewidth=\hsize\raggedright\arraybackslash}X>{\hsize=1.1538\hsize\linewidth=\hsize\raggedright\arraybackslash}X>{\hsize=1.1538\hsize\linewidth=\hsize\raggedright\arraybackslash}X>{\hsize=1.1538\hsize\linewidth=\hsize\raggedright\arraybackslash}X@{}}
\toprule
Deleted $m$ & Highest margin & Lowest margin & Random (5 draws)\\
\midrule
0 & \metric{0.8561}{0.0017} & \metric{0.8561}{0.0017} & \metric{0.8561}{0.0017}\\
1 & \metric{0.8565}{0.0004} & \metric{0.8547}{0.0008} & \metric{0.8552}{0.0007}\\
2 & \metric{0.8563}{0.0001} & \metric{0.8539}{0.0004} & \metric{0.8548}{0.0008}\\
5 & \metric{0.8583}{0.0002} & \metric{0.8530}{0.0004} & \metric{0.8544}{0.0008}\\
10 & \metric{0.8568}{0.0003} & \metric{0.8492}{0.0013} & \metric{0.8543}{0.0007}\\
15 & \metric{0.8466}{0.0032} & \metric{0.8459}{0.0013} & \metric{0.8508}{0.0001}\\
20 & \metric{0.8362}{0.0039} & \metric{0.8354}{0.0041} & \metric{0.8439}{0.0010}\\
25 & \metric{0.8070}{0.0014} & \metric{0.8170}{0.0063} & \metric{0.8276}{0.0028}\\
30 & \metric{0.5702}{0.0063} & \metric{0.5702}{0.0063} & \metric{0.5702}{0.0063}\\
\bottomrule\end{tabularx}
\Note{Selection and checkpoint are frozen. Mean $\pm$ standard deviation over model seeds; random draws are averaged within each seed. Static covariates remain at all $m$.}
\end{table}
\begin{table}[!htbp]
\ContinuedFloat
\centering
\caption{Evidence deletion (continued): (e) MIMIC-III test AUROC.}
\label{tab:deletion_auroc_mimiciii}
\footnotesize
\setlength{\tabcolsep}{1.0pt}\renewcommand{\arraystretch}{1.16}
\begin{tabularx}{\linewidth}{@{}>{\hsize=0.5385\hsize\linewidth=\hsize\raggedright\arraybackslash}X>{\hsize=1.1538\hsize\linewidth=\hsize\raggedright\arraybackslash}X>{\hsize=1.1538\hsize\linewidth=\hsize\raggedright\arraybackslash}X>{\hsize=1.1538\hsize\linewidth=\hsize\raggedright\arraybackslash}X@{}}
\toprule
Deleted $m$ & Highest margin & Lowest margin & Random (5 draws)\\
\midrule
0 & \metric{0.8563}{0.0024} & \metric{0.8563}{0.0024} & \metric{0.8563}{0.0024}\\
1 & \metric{0.8567}{0.0024} & \metric{0.8550}{0.0026} & \metric{0.8550}{0.0024}\\
2 & \metric{0.8574}{0.0027} & \metric{0.8547}{0.0027} & \metric{0.8543}{0.0024}\\
5 & \metric{0.8567}{0.0028} & \metric{0.8544}{0.0039} & \metric{0.8544}{0.0028}\\
10 & \metric{0.8514}{0.0016} & \metric{0.8527}{0.0044} & \metric{0.8517}{0.0029}\\
15 & \metric{0.8391}{0.0015} & \metric{0.8506}{0.0061} & \metric{0.8484}{0.0036}\\
20 & \metric{0.8291}{0.0063} & \metric{0.8433}{0.0079} & \metric{0.8408}{0.0047}\\
25 & \metric{0.8054}{0.0091} & \metric{0.8214}{0.0141} & \metric{0.8214}{0.0081}\\
30 & \metric{0.5006}{0.0136} & \metric{0.5006}{0.0136} & \metric{0.5006}{0.0136}\\
\bottomrule\end{tabularx}
\Note{Selection and checkpoint are frozen. Mean $\pm$ standard deviation over model seeds; random draws are averaged within each seed. Static covariates remain at all $m$.}
\end{table}
\begin{table}[!htbp]
\ContinuedFloat
\centering
\caption{Evidence deletion (continued): (f) P2019 test AUROC.}
\label{tab:deletion_auroc_p2019}
\footnotesize
\setlength{\tabcolsep}{1.0pt}\renewcommand{\arraystretch}{1.16}
\begin{tabularx}{\linewidth}{@{}>{\hsize=0.5385\hsize\linewidth=\hsize\raggedright\arraybackslash}X>{\hsize=1.1538\hsize\linewidth=\hsize\raggedright\arraybackslash}X>{\hsize=1.1538\hsize\linewidth=\hsize\raggedright\arraybackslash}X>{\hsize=1.1538\hsize\linewidth=\hsize\raggedright\arraybackslash}X@{}}
\toprule
Deleted $m$ & Highest margin & Lowest margin & Random (5 draws)\\
\midrule
0 & \metric{0.9115}{0.0016} & \metric{0.9115}{0.0016} & \metric{0.9115}{0.0016}\\
1 & \metric{0.9104}{0.0026} & \metric{0.9111}{0.0022} & \metric{0.9111}{0.0018}\\
2 & \metric{0.9088}{0.0041} & \metric{0.9111}{0.0020} & \metric{0.9105}{0.0019}\\
5 & \metric{0.9055}{0.0069} & \metric{0.9101}{0.0023} & \metric{0.9094}{0.0024}\\
10 & \metric{0.8893}{0.0136} & \metric{0.9076}{0.0024} & \metric{0.9061}{0.0029}\\
15 & \metric{0.8709}{0.0171} & \metric{0.9050}{0.0022} & \metric{0.9014}{0.0038}\\
20 & \metric{0.8421}{0.0198} & \metric{0.9003}{0.0024} & \metric{0.8912}{0.0054}\\
25 & \metric{0.7948}{0.0167} & \metric{0.8851}{0.0036} & \metric{0.8635}{0.0048}\\
30 & \metric{0.4831}{0.0277} & \metric{0.4831}{0.0277} & \metric{0.4831}{0.0277}\\
\bottomrule\end{tabularx}
\Note{Selection and checkpoint are frozen. Mean $\pm$ standard deviation over model seeds; random draws are averaged within each seed. Static covariates remain at all $m$.}
\end{table}
