# Supplementary material for: Learning to Select Source-Traceable Evidence for Language-Model Prediction from Irregular Clinical Time Series
Source: arXiv:2605.20292 source file (2026-09-30)
Supplement: Supplementary file 3 [file table_xgb_validation.tex]

\begin{table}[!htbp]
\centering
\caption{Validation AUROC for the same \textsc{XGB-WindowStats} fits as Table~\ref{tab:xgb_sweep}: mean $\pm$ standard deviation over seeds 0, 1, and 2.}
\label{tab:xgb_validation}
\footnotesize
\setlength{\tabcolsep}{1pt}\renewcommand{\arraystretch}{1.15}
\begin{tabular*}{\linewidth}{@{\extracolsep{\fill}}l*{3}{c}@{}}
\toprule
Max. trees $n$ & P2012 & MIMIC-III & P2019\\
\midrule
1 & \metric{0.7588}{0.0044} & \metric{0.7914}{0.0076} & \metric{0.7797}{0.0009}\\
5 & \metric{0.8158}{0.0036} & \metric{0.8264}{0.0034} & \metric{0.8602}{0.0022}\\
10 & \metric{0.8323}{0.0007} & \metric{0.8330}{0.0020} & \metric{0.8735}{0.0009}\\
15 & \metric{0.8401}{0.0019} & \metric{0.8360}{0.0021} & \metric{0.8769}{0.0035}\\
20 & \metric{0.8422}{0.0019} & \metric{0.8388}{0.0013} & \metric{0.8821}{0.0010}\\
25 & \metric{0.8454}{0.0030} & \metric{0.8405}{0.0016} & \metric{0.8844}{0.0013}\\
30 & \metric{0.8472}{0.0026} & \metric{0.8435}{0.0008} & \metric{0.8854}{0.0024}\\
35 & \metric{0.8500}{0.0024} & \metric{0.8454}{0.0015} & \metric{0.8868}{0.0019}\\
40 & \metric{0.8519}{0.0028} & \metric{0.8468}{0.0013} & \metric{0.8891}{0.0021}\\
60 & \metric{0.8550}{0.0026} & \metric{0.8522}{0.0013} & \metric{0.8970}{0.0010}\\
100 & \metric{0.8616}{0.0011} & \textbf{\metric{0.8594}{0.0014}} & \textbf{\metric{0.9179}{0.0010}}\\
200 & \textbf{\metric{0.8663}{0.0016}} & \metric{0.8561}{0.0022} & \metric{0.9175}{0.0021}\\
\bottomrule
\end{tabular*}
\Note{Bold marks the highest mean validation AUROC in each dataset. One common cap is selected across the three seeds per dataset; all corresponding test results, rather than a best seed, are summarized in the tuned row of Table~\ref{tab:xgb}.}
\end{table}
